# Supplementary material for: Approaching Chemical Accuracy with Quantum Monte Carlo
Source: arXiv:1202.0317 source file (2012-02-01)
Supplement: Supplementary file 1 [file supplementary.pdf]

# Supplementary Material

F. R. Petruzielo, Julien Toulouse, C. J. Umrigar  
(Dated: January 31, 2012)

## 1 Hydrogen Pseudopotential and Basis Sets

A significantly improved hydrogen pseudopotential developed by Filippi and Dolg is provided in Table 1. The  $s$  contraction for the hydrogen basis sets is given in Table 2. The Gauss-Slater (GS) primitives for the double-zeta ( $2z$ ) atomic natural orbital GS (ANO-GS) basis for hydrogen are provided in Table 3. The GS primitives for the triple-zeta ( $3z$ ) ANO-GS basis for hydrogen are provided in Table 4. The Gaussian primitives for the quintuple-zeta ( $5z$ ) Gaussian basis for hydrogen are provided in Table 5. Each basis was constructed using the methods of Ref. [1].

Table 1: Significantly improved pseudopotential for hydrogen developed by Filippi and Dolg to replace pseudopotential from Ref. [2, 3]. Format is appropriate for GAMESS [4].

| H-QMC GEN 0 1   |   |                 |
|-----------------|---|-----------------|
| 3               |   |                 |
| 1.00000000      | 1 | 10.             |
| 10.             | 3 | 9.872559446615  |
| -7.556924974646 | 2 | 10.258560602196 |

Table 2:  $s$  contraction for hydrogen basis sets. The contraction was constructed using the method of Ref. [1].

| Exponent    | Coefficient |
|-------------|-------------|
| 0.05559917  | 0.070858475 |
| 0.11675826  | 0.283134279 |
| 0.24519235  | 0.347654627 |
| 0.51490394  | 0.233232914 |
| 1.08129828  | 0.119346810 |
| 2.27072639  | 0.053366645 |
| 4.76852541  | 0.022054957 |
| 10.01390336 | 0.011743843 |
| 21.02919706 | 0.000820785 |

Table 3: Primitives for  $2z$  ANO-GS basis for hydrogen. The primitives were constructed using the method of Ref. [1].

| Function | Exp.     |
|----------|----------|
| GS-1S    | 1.946875 |
| GS-2P    | 1.968750 |

Table 4: Primitives for 3z ANO-GS basis for hydrogen. The primitives were constructed using the method of Ref. [1].

| Function | Exp.     |
|----------|----------|
| GS-1S    | 0.925000 |
| GS-1S    | 1.968750 |
| GS-2P    | 1.887500 |
| GS-2P    | 2.553125 |
| GS-3D    | 2.659375 |

Table 5: Primitives for 5z Gaussian basis for hydrogen. The primitives were constructed using the method of Ref. [1].

| Function | Exp.      |
|----------|-----------|
| 1S       | 0.0692135 |
| 1S       | 0.1736131 |
| 1S       | 0.4543641 |
| 1S       | 1.3072524 |
| 2P       | 0.2370069 |
| 2P       | 0.6258464 |
| 2P       | 1.6114234 |
| 2P       | 5.1965679 |
| 3D       | 0.5106775 |
| 3D       | 1.3660613 |
| 3D       | 3.2652161 |
| 4F       | 0.6792030 |
| 4F       | 2.0042817 |

## 2 Setup and Reference Data

The geometries, zero point energies, and experimental atomization energies for the molecules of the G2 set [5] are provided in Table 6.

Table 6: Geometries, zero point energies, and experimental atomization energies for the molecules of the G2 set [5]. Some experimental error bars were not available (N/A).

| System                                           | Geometry | ZPE (kcal/mol) | Expt. Atomization Energy (kcal/mol) |
|--------------------------------------------------|----------|----------------|-------------------------------------|
| LiH                                              | [6]      | 1.99 [6]       | $56 \pm 0.01$ [7]                   |
| BeH                                              | [6]      | 2.92 [6]       | $46.9 \pm 0.01$ [7]                 |
| CH                                               | [6]      | 4.04 [6]       | $79.9 \pm 0.02$ [7]                 |
| CH <sub>2</sub> ( <sup>3</sup> B <sub>1</sub> )  | [6]      | 10.55 [6]      | $179.6 \pm \text{N/A}$ [7]          |
| CH <sub>2</sub> ( <sup>1</sup> A <sub>1</sub> )  | [6]      | 10.29 [6]      | $170.6 \pm \text{N/A}$ [7]          |
| CH <sub>3</sub>                                  | [6]      | 18.55 [6]      | $289.3 \pm 0.2$ [7]                 |
| CH <sub>4</sub>                                  | [6]      | 27.74 [6]      | $392.5 \pm 0.1$ [7]                 |
| NH                                               | [6]      | 4.64 [6]       | $79 \pm 0.4$ [7]                    |
| NH <sub>2</sub>                                  | [6]      | 11.84 [6]      | $170 \pm 0.3$ [7]                   |
| NH <sub>3</sub>                                  | [6]      | 21.33 [6]      | $276.7 \pm 0.1$ [7]                 |
| OH                                               | [6]      | 5.29 [6]       | $101.4 \pm 0.3$ [7]                 |
| H <sub>2</sub> O                                 | [6]      | 13.26 [6]      | $219.35 \pm 0.01$ [7]               |
| HF                                               | [6]      | 5.86 [6]       | $135.2 \pm 0.2$ [7]                 |
| SiH <sub>2</sub> ( <sup>1</sup> A <sub>1</sub> ) | [8]      | 7.3 [7]        | $144.4 \pm 0.7$ [7]                 |
| SiH <sub>2</sub> ( <sup>3</sup> B <sub>1</sub> ) | [9]      | 7.5 [7]        | $123.4 \pm 0.7$ [7]                 |
| SiH <sub>3</sub>                                 | [8]      | 13.2 [7]       | $213.8 \pm 1.2$ [7]                 |
| SiH <sub>4</sub>                                 | [8]      | 19.4 [7]       | $302.6 \pm 0.5$ [7]                 |
| PH <sub>2</sub>                                  | [8]      | 8.4 [7]        | $144.7 \pm 0.6$ [7]                 |
| PH <sub>3</sub>                                  | [6]      | 14.44 [6]      | $228.6 \pm 0.4$ [7]                 |
| H <sub>2</sub> S                                 | [6]      | 9.4 [6]        | $173.1 \pm 0.2$ [7]                 |
| HCl                                              | [6]      | 4.24 [6]       | $102.24 \pm 0.5$ [7]                |
| Li <sub>2</sub>                                  | [10]     | 0.5 [6]        | $23.9 \pm 0.7$ [7]                  |
| LiF                                              | [10]     | 1.3 [7]        | $137.6 \pm 2$ [7]                   |
| C <sub>2</sub> H <sub>2</sub>                    | [6]      | 16.5 [6]       | $386.9 \pm 0.2$ [7]                 |
| C <sub>2</sub> H <sub>4</sub>                    | [6]      | 31.66 [6]      | $531.9 \pm 0.1$ [7]                 |
| C <sub>2</sub> H <sub>6</sub>                    | [6]      | 46.23 [6]      | $666.3 \pm \text{N/A}$ [7]          |
| CN                                               | [6]      | 2.95 [6]       | $178.1 \pm 2.4$ [7]                 |
| HCN                                              | [6]      | 9.95 [6]       | $301.7 \pm 2$ [7]                   |
| CO                                               | [6]      | 3.09 [6]       | $256.2 \pm 0.2$ [7]                 |
| HCO                                              | [6]      | 8.09 [6]       | $270.3 \pm 2$ [7]                   |
| H <sub>2</sub> CO                                | [6]      | 16.52 [6]      | $357.2 \pm 0.1$ [7]                 |
| H <sub>3</sub> COH                               | [8]      | 31.72 [6]      | $480.8 \pm \text{N/A}$ [7]          |
| N <sub>2</sub>                                   | [6]      | 3.36 [6]       | $225.1 \pm 0.4$ [7]                 |
| N <sub>2</sub> H <sub>4</sub>                    | [8]      | 32.68 [6]      | $405.4 \pm \text{N/A}$ [7]          |
| NO                                               | [6]      | 2.71 [6]       | $150.06 \pm 0.04$ [7]               |
| O <sub>2</sub>                                   | [10]     | 2.25 [6]       | $117.96 \pm 0.02$ [7]               |
| H <sub>2</sub> O <sub>2</sub>                    | [6]      | 16.44 [6]      | $252.3 \pm \text{N/A}$ [7]          |
| F <sub>2</sub>                                   | [10]     | 1.3 [6]        | $36.9 \pm 0.1$ [7]                  |
| CO <sub>2</sub>                                  | [6]      | 7.24 [6]       | $381.93 \pm 0.01$ [7]               |
| Na <sub>2</sub>                                  | [8]      | 0.2 [7]        | $16.8 \pm 0.3$ [7]                  |
| Si <sub>2</sub>                                  | [10]     | 0.73 [6]       | $74 \pm \text{N/A}$ [7]             |
| P <sub>2</sub>                                   | [10]     | 1.11 [6]       | $116.1 \pm 0.5$ [7]                 |

Table 6 – continued

| System                         | Geometry | ZPE (kcal/mol) | Expt. Atomization Energy (kcal/mol) |
|--------------------------------|----------|----------------|-------------------------------------|
| S <sub>2</sub>                 | [10]     | 1.04 [6]       | 100.66 ± 0.07 [7]                   |
| Cl <sub>2</sub>                | [6]      | 0.8 [6]        | 57.18 ± 0.01 [7]                    |
| NaCl                           | [8]      | 0.5 [7]        | 97.3 ± 0.5 [7]                      |
| SiO                            | [6]      | 1.78 [6]       | 189.9 ± 2 [7]                       |
| CS                             | [10]     | 1.83 [6]       | 169.4 ± 6 [7]                       |
| SO                             | [6]      | 1.63 [6]       | 123.4 ± 0.3 [7]                     |
| ClO                            | [10]     | 1.22 [6]       | 63.42 ± 0.02 [7]                    |
| ClF                            | [6]      | 1.12 [6]       | 60.4 ± N/A [7]                      |
| Si <sub>2</sub> H <sub>6</sub> | [8]      | 30.5 [7]       | 500.1 ± N/A [7]                     |
| CH <sub>3</sub> Cl             | [6]      | 23.19 [6]      | 371 ± N/A [7]                       |
| H <sub>3</sub> CSH             | [8]      | 28.6 [7]       | 445.1 ± N/A [7]                     |
| HOCl                           | [6]      | 8.18 [6]       | 156.3 ± 0.5 [7]                     |
| SO <sub>2</sub>                | [10]     | 4.38 [6]       | 254 ± 0.2 [7]                       |

### 3 Raw Data

#### 3.1 Locality Approximation

This section contains the raw data for those systems handled with the locality approximation [11]. The diffusion Monte Carlo (DMC) total energies of the molecules from the G2 set and their atoms for a single determinant Slater-Jastrow (SJ) trial wavefunction composed of Hartree-Fock (HF) orbitals are given in Table 7. The DMC total energies of the molecules from the G2 set and their atoms for a single determinant SJ trial wavefunction composed of variational Monte Carlo (VMC) optimized orbitals are given in Table 8. The DMC total energies of the molecules from the G2 set and their atoms for a CAS SJ trial wavefunction with an  $s$  and  $p$  active space are given in Table 9. The DMC total energies of the phosphorus containing molecules from the G2 set and their atoms for a single determinant SJ trial wavefunction composed of VMC optimized orbitals, a CAS SJ trial wavefunction with an  $s$  and  $p$  active space, and a CAS SJ trial wavefunction with an  $s$ ,  $p$ , and  $d$  active space are given in Table 10.

Table 7: DMC total energies of the molecules from the G2 set and their atoms for a single determinant SJ trial wavefunction composed of HF orbitals. Energies are in Hartrees. Error bar, which is shown in parentheses, is for the last digit.

| System                                          | 2z            | 3z            | 5z            |
|-------------------------------------------------|---------------|---------------|---------------|
| H                                               | -0.5000006(1) | -0.5000006(1) | -0.5000006(1) |
| Li                                              | -0.1963297(5) | -0.1963297(7) | -0.196329(2)  |
| C                                               | -5.42251(7)   | -5.42233(8)   | -5.42236(7)   |
| N                                               | -9.79127(7)   | -9.79109(5)   | -9.79123(6)   |
| O                                               | -15.89289(8)  | -15.89228(8)  | -15.89254(8)  |
| F                                               | -24.18633(8)  | -24.18594(7)  | -24.18609(7)  |
| Na                                              | -0.1821457(7) | -0.1821441(7) | -0.182145(2)  |
| Si                                              | -3.76661(5)   | -3.76662(5)   | -3.76654(5)   |
| P                                               | -6.47660(7)   | -6.47648(5)   | -6.47645(7)   |
| S                                               | -10.13125(9)  | -10.13103(9)  | -10.1311(1)   |
| Cl                                              | -14.97223(6)  | -14.97168(6)  | -14.97179(6)  |
| CH                                              | -6.05266(7)   | -6.05399(9)   | -6.05422(8)   |
| CH <sub>2</sub> ( <sup>1</sup> A <sub>1</sub> ) | -6.7061(1)    | -6.70751(9)   | -6.70792(9)   |
| CH <sub>3</sub>                                 | -7.41421(9)   | -7.41476(8)   | -7.41490(8)   |

Table 7 – continued

| System                                           | 2z           | 3z           | 5z           |
|--------------------------------------------------|--------------|--------------|--------------|
| CH <sub>4</sub>                                  | -8.09421(9)  | -8.09441(9)  | -8.09451(8)  |
| NH                                               | -10.41946(8) | -10.42028(7) | -10.42068(8) |
| NH <sub>2</sub>                                  | -11.07601(9) | -11.07774(9) | -11.07834(9) |
| NH <sub>3</sub>                                  | -11.7593(1)  | -11.76181(8) | -11.76266(9) |
| OH                                               | -16.56031(9) | -16.56126(9) | -16.56142(9) |
| H <sub>2</sub> O                                 | -17.25949(8) | -17.26123(8) | -17.26175(9) |
| HF                                               | -24.90895(8) | -24.91024(7) | -24.91083(8) |
| SiH <sub>2</sub> ( <sup>1</sup> A <sub>1</sub> ) | -5.00856(7)  | -5.00925(7)  | -5.00952(7)  |
| SiH <sub>2</sub> ( <sup>3</sup> B <sub>1</sub> ) | -4.97656(7)  | -4.97723(7)  | -4.97709(6)  |
| SiH <sub>3</sub>                                 | -5.6280(1)   | -5.62910(8)  | -5.62906(9)  |
| SiH <sub>4</sub>                                 | -6.28261(9)  | -6.28418(8)  | -6.28428(7)  |
| PH <sub>2</sub>                                  | -7.71744(8)  | -7.71798(8)  | -7.71812(8)  |
| PH <sub>3</sub>                                  | -8.35619(7)  | -8.35676(7)  | -8.35696(7)  |
| H <sub>2</sub> S                                 | -11.41932(8) | -11.41962(7) | -11.42012(7) |
| HCl                                              | -15.64183(8) | -15.64178(8) | -15.64211(8) |
| Li <sub>2</sub>                                  | -0.43045(2)  | -0.43053(3)  | -0.43053(2)  |
| C <sub>2</sub> H <sub>4</sub>                    | -13.74229(8) | -13.7433(1)  | -13.74348(8) |
| C <sub>2</sub> H <sub>6</sub>                    | -14.98415(8) | -14.9851(1)  | -14.9850(1)  |
| CO                                               | -21.7192(1)  | -21.7232(1)  | -21.7238(1)  |
| H <sub>2</sub> CO                                | -22.9038(1)  | -22.9080(1)  | -22.9082(1)  |
| H <sub>3</sub> COH                               | -24.12892(9) | -24.13207(8) | -24.13271(8) |
| N <sub>2</sub>                                   | -19.9296(1)  | -19.9333(1)  | -19.9338(1)  |
| N <sub>2</sub> H <sub>4</sub>                    | -22.26561(9) | -22.27033(9) | -22.27206(8) |
| NO                                               | -25.9062(1)  | -25.9108(1)  | -25.9117(1)  |
| O <sub>2</sub>                                   | -31.9642(1)  | -31.9679(1)  | -31.9691(1)  |
| H <sub>2</sub> O <sub>2</sub>                    | -33.1973(1)  | -33.2013(1)  | -33.2025(1)  |
| F <sub>2</sub>                                   | -48.4134(1)  | -48.4146(1)  | -48.41757(9) |
| CO <sub>2</sub>                                  | -37.8168(1)  | -37.8228(1)  | -37.8235(1)  |
| Na <sub>2</sub>                                  | -0.39102(2)  | -0.39106(2)  | -0.39104(2)  |
| Si <sub>2</sub>                                  | -7.6498(1)   | -7.6505(1)   | -7.65031(9)  |
| P <sub>2</sub>                                   | -13.1256(1)  | -13.1273(1)  | -13.1275(1)  |
| S <sub>2</sub>                                   | -20.4191(1)  | -20.4207(1)  | -20.4214(1)  |
| Cl <sub>2</sub>                                  | -30.0309(1)  | -30.0305(1)  | -30.03165(9) |
| SiO                                              | -19.9535(1)  | -19.96031(9) | -19.96104(8) |
| CS                                               | -15.8151(1)  | -15.8169(1)  | -15.8185(1)  |
| SO                                               | -26.2105(1)  | -26.2159(1)  | -26.21669(9) |
| ClO                                              | -30.9457(1)  | -30.9475(1)  | -30.9486(1)  |
| ClF                                              | -39.2434(1)  | -39.24608(9) | -39.2478(1)  |
| Si <sub>2</sub> H <sub>6</sub>                   | -11.3836(1)  | -11.3857(1)  | -11.38579(9) |
| CH <sub>3</sub> Cl                               | -22.5236(1)  | -22.5245(1)  | -22.5249(1)  |
| H <sub>3</sub> CSH                               | -18.30598(9) | -18.3071(1)  | -18.30752(9) |
| HOCl                                             | -31.61547(9) | -31.6179(1)  | -31.6193(1)  |
| SO <sub>2</sub>                                  | -42.2986(1)  | -42.3125(1)  | -42.3152(1)  |

Table 8: The DMC total energies of the molecules from the G2 set and their atoms for a single determinant SJ trial wavefunction composed of VMC optimized orbitals. Energies are in Hartrees. Error bar, which is shown in parentheses, is for the last digit.

| System                                           | 2z            | 3z            | 5z            |
|--------------------------------------------------|---------------|---------------|---------------|
| H                                                | -0.5000005(1) | -0.5000006(1) | -0.5000005(1) |
| Li                                               | -0.1963295(4) | -0.1963292(4) | -0.1963296(3) |
| C                                                | -5.42288(7)   | -5.42292(7)   | -5.42296(6)   |
| N                                                | -9.79213(6)   | -9.79230(6)   | -9.79229(6)   |
| O                                                | -15.8930(1)   | -15.89305(8)  | -15.89310(7)  |
| F                                                | -24.18619(5)  | -24.18651(7)  | -24.18636(8)  |
| Na                                               | -0.1821438(7) | -0.1821446(4) | -0.1821438(4) |
| Si                                               | -3.76682(5)   | -3.76676(4)   | -3.76683(4)   |
| P                                                | -6.47688(9)   | -6.47699(5)   | -6.47686(5)   |
| S                                                | -10.1317(1)   | -10.13184(8)  | -10.13189(7)  |
| Cl                                               | -14.97253(6)  | -14.97252(6)  | -14.97261(6)  |
| CH                                               | -6.05388(8)   | -6.05473(7)   | -6.05476(9)   |
| CH <sub>2</sub> ( <sup>1</sup> A <sub>1</sub> )  | -6.70711(9)   | -6.70861(8)   | -6.70860(7)   |
| CH <sub>3</sub>                                  | -7.41489(7)   | -7.41544(9)   | -7.41549(7)   |
| CH <sub>4</sub>                                  | -8.09523(7)   | -8.09523(8)   | -8.09523(8)   |
| NH                                               | -10.42146(8)  | -10.42200(8)  | -10.42186(7)  |
| NH <sub>2</sub>                                  | -11.07824(9)  | -11.07960(8)  | -11.07962(8)  |
| NH <sub>3</sub>                                  | -11.76205(8)  | -11.76368(7)  | -11.76378(7)  |
| OH                                               | -16.56188(9)  | -16.56243(8)  | -16.56264(9)  |
| H <sub>2</sub> O                                 | -17.26195(8)  | -17.26298(8)  | -17.26313(8)  |
| HF                                               | -24.91098(7)  | -24.91170(6)  | -24.91175(7)  |
| SiH <sub>2</sub> ( <sup>1</sup> A <sub>1</sub> ) | -5.00947(5)   | -5.01034(5)   | -5.01055(4)   |
| SiH <sub>2</sub> ( <sup>3</sup> B <sub>1</sub> ) | -4.97846(4)   | -4.97932(3)   | -4.97952(3)   |
| SiH <sub>3</sub>                                 | -5.62975(6)   | -5.63077(6)   | -5.63097(5)   |
| SiH <sub>4</sub>                                 | -6.28405(6)   | -6.28526(5)   | -6.28548(5)   |
| PH <sub>2</sub>                                  | -7.71870(8)   | -7.71952(6)   | -7.71994(6)   |
| PH <sub>3</sub>                                  | -8.35790(7)   | -8.35892(5)   | -8.35921(6)   |
| H <sub>2</sub> S                                 | -11.42111(8)  | -11.42203(7)  | -11.42238(7)  |
| HCl                                              | -15.64294(7)  | -15.64345(7)  | -15.64374(7)  |
| Li <sub>2</sub>                                  | -0.43069(2)   | -0.43069(5)   | -0.43077(4)   |
| C <sub>2</sub> H <sub>4</sub>                    | -13.74413(7)  | -13.74453(6)  | -13.74477(7)  |
| C <sub>2</sub> H <sub>6</sub>                    | -14.98622(7)  | -14.98643(7)  | -14.98640(6)  |
| CO                                               | -21.72262(9)  | -21.72572(9)  | -21.72617(9)  |
| H <sub>2</sub> CO                                | -22.9080(1)   | -22.91048(9)  | -22.91083(9)  |
| H <sub>3</sub> COH                               | -24.13189(8)  | -24.13417(7)  | -24.1348(1)   |
| N <sub>2</sub>                                   | -19.93256(9)  | -19.93600(9)  | -19.93638(9)  |
| N <sub>2</sub> H <sub>4</sub>                    | -22.26927(9)  | -22.27373(7)  | -22.27469(8)  |
| NO                                               | -25.9119(1)   | -25.91612(9)  | -25.91693(9)  |
| O <sub>2</sub>                                   | -31.9682(1)   | -31.9707(1)   | -31.9719(1)   |
| H <sub>2</sub> O <sub>2</sub>                    | -33.2030(1)   | -33.20627(8)  | -33.20778(9)  |
| F <sub>2</sub>                                   | -48.4216(1)   | -48.42302(9)  | -48.42522(8)  |
| CO <sub>2</sub>                                  | -37.8259(1)   | -37.8287(1)   | -37.8291(1)   |
| Na <sub>2</sub>                                  | -0.39104(1)   | -0.39104(4)   | -0.39106(2)   |
| Si <sub>2</sub>                                  | -7.65138(6)   | -7.65274(8)   | -7.65279(7)   |
| P <sub>2</sub>                                   | -13.12785(9)  | -13.1300(1)   | -13.13077(9)  |
| S <sub>2</sub>                                   | -20.4211(1)   | -20.4236(1)   | -20.4248(1)   |

Table 8 – continued

| System                         | 2z           | 3z           | 5z           |
|--------------------------------|--------------|--------------|--------------|
| Cl <sub>2</sub>                | -30.03397(9) | -30.03514(9) | -30.03684(8) |
| SiO                            | -19.95896(9) | -19.96336(9) | -19.96385(7) |
| CS                             | -15.81932(9) | -15.82302(9) | -15.82387(8) |
| SO                             | -26.21600(9) | -26.22047(9) | -26.22172(9) |
| ClO                            | -30.9600(1)  | -30.96312(9) | -30.96463(9) |
| ClF                            | -39.24935(9) | -39.25234(7) | -39.25406(8) |
| Si <sub>2</sub> H <sub>6</sub> | -11.38585(8) | -11.38818(7) | -11.38840(7) |
| CH <sub>3</sub> Cl             | -22.5259(1)  | -22.5266(1)  | -22.5275(1)  |
| H <sub>3</sub> CSH             | -18.30852(9) | -18.30988(8) | -18.31105(7) |
| HOCl                           | -31.62113(9) | -31.62387(9) | -31.62501(8) |
| SO <sub>2</sub>                | -42.3125(1)  | -42.32256(8) | -42.32431(8) |

Table 9: The DMC total energies of the molecules from the G2 set and their atoms for a CAS SJ trial wavefunction with an *s* and *p* active space. Energies are in Hartrees. Error bar, which is shown in parentheses, is for the last digit.

| System                                           | 3z            |
|--------------------------------------------------|---------------|
| H                                                | -0.5000006(1) |
| Li                                               | -0.1963292(4) |
| C                                                | -5.42823(6)   |
| N                                                | -9.79230(6)   |
| O                                                | -15.89305(8)  |
| F                                                | -24.18651(7)  |
| Na                                               | -0.1821446(4) |
| Si                                               | -3.76711(4)   |
| P                                                | -6.47699(5)   |
| S                                                | -10.13184(8)  |
| Cl                                               | -14.97252(6)  |
| CH                                               | -6.06239(6)   |
| CH <sub>2</sub> ( <sup>1</sup> A <sub>1</sub> )  | -6.71713(6)   |
| CH <sub>3</sub>                                  | -7.41764(6)   |
| CH <sub>4</sub>                                  | -8.09730(6)   |
| NH                                               | -10.42390(7)  |
| NH <sub>2</sub>                                  | -11.08219(7)  |
| NH <sub>3</sub>                                  | -11.76623(6)  |
| OH                                               | -16.56411(8)  |
| H <sub>2</sub> O                                 | -17.26521(7)  |
| HF                                               | -24.91286(7)  |
| SiH <sub>2</sub> ( <sup>1</sup> A <sub>1</sub> ) | -5.01238(4)   |
| SiH <sub>2</sub> ( <sup>3</sup> B <sub>1</sub> ) | -4.97970(3)   |
| SiH <sub>3</sub>                                 | -5.63114(4)   |
| SiH <sub>4</sub>                                 | -6.28571(4)   |
| PH <sub>2</sub>                                  | -7.72051(5)   |
| PH <sub>3</sub>                                  | -8.36003(5)   |
| H <sub>2</sub> S                                 | -11.42305(7)  |
| HCl                                              | -15.64382(5)  |
| Li <sub>2</sub>                                  | -0.431584(5)  |
| C <sub>2</sub> H <sub>4</sub>                    | -13.75239(8)  |

Table 9 – continued

| System                         | 3z           |
|--------------------------------|--------------|
| C <sub>2</sub> H <sub>6</sub>  | -14.99037(9) |
| CO                             | -21.73788(7) |
| H <sub>2</sub> CO              | -22.9190(1)  |
| H <sub>3</sub> COH             | -24.14011(5) |
| N <sub>2</sub>                 | -19.95032(7) |
| N <sub>2</sub> H <sub>4</sub>  | -22.27934(5) |
| NO                             | -25.92787(8) |
| O <sub>2</sub>                 | -31.97692(9) |
| H <sub>2</sub> O <sub>2</sub>  | -33.21410(9) |
| F <sub>2</sub>                 | -48.43320(8) |
| CO <sub>2</sub>                | -37.83890(7) |
| Na <sub>2</sub>                | -0.39106(2)  |
| Si <sub>2</sub>                | -7.65485(7)  |
| P <sub>2</sub>                 | -13.13441(8) |
| S <sub>2</sub>                 | -20.42452(9) |
| Cl <sub>2</sub>                | -30.03679(9) |
| SiO                            | -19.96885(7) |
| CS                             | -15.83223(6) |
| SO                             | -26.22235(9) |
| ClO                            | -30.96605(8) |
| ClF                            | -39.25596(7) |
| Si <sub>2</sub> H <sub>6</sub> | -11.38838(7) |
| CH <sub>3</sub> Cl             | -22.52839(7) |
| H <sub>3</sub> CSH             | -18.3128(1)  |
| HOCl                           | -31.6278(1)  |
| SO <sub>2</sub>                | -42.33049(6) |

Table 10: The DMC total energies of the phosphorus containing molecules from the G2 set and their atoms for a single determinant SJ trial wavefunction composed of VMC optimized orbitals, a CAS SJ trial wavefunction with an  $s$  and  $p$  active space, and a CAS SJ trial wavefunction with an  $s$ ,  $p$ , and  $d$  active space. Energies are in Hartrees. Error bar, which is shown in parentheses, is for the last digit.

| System          | 1CSF          | $s, p$ CAS    | $s, p, d$ CAS |
|-----------------|---------------|---------------|---------------|
| H               | -0.5000006(1) | -0.5000006(1) | -0.5000006(1) |
| P               | -6.47699(5)   | -6.47699(5)   | -6.47753(5)   |
| PH <sub>2</sub> | -7.71952(6)   | -7.72051(5)   | -7.72183(5)   |
| PH <sub>3</sub> | -8.35892(5)   | -8.36003(5)   | -8.36145(6)   |
| P <sub>2</sub>  | -13.1300(1)   | -13.13441(8)  | -13.13814(7)  |

### 3.2 T-Moves

This section contains the raw data for those systems handled with the size-consistent version of T-Moves [12]. The DMC total energies of the molecules from the G2 set and their atoms for a single determinant SJ trial wavefunction composed of HF orbitals are given in Table 11. The DMC total energies of the molecules from the G2 set and their atoms for a single determinant SJ trial wavefunction composed of VMC optimized

orbitals are given in Table 12. The DMC total energies of the molecules from the G2 set and their atoms for a CAS SJ trial wavefunction with an  $s$  and  $p$  active space are given in Table 13.

Table 11: DMC total energies of the molecules from the G2 set and their atoms for a single determinant SJ trial wavefunction composed of HF orbitals. Energies are in Hartrees. Error bar, which is shown in parentheses, is for the last digit.

| System                                          | 2z            | 3z            | 5z            |
|-------------------------------------------------|---------------|---------------|---------------|
| H                                               | -0.5000006(1) | -0.5000006(1) | -0.5000006(1) |
| Li                                              | -0.1963297(5) | -0.1963297(7) | -0.196329(2)  |
| Be                                              | -1.00918(5)   | -1.00928(4)   | -1.00926(5)   |
| C                                               | -5.42211(7)   | -5.42206(7)   | -5.42194(6)   |
| N                                               | -9.79121(5)   | -9.79092(6)   | -9.79123(6)   |
| O                                               | -15.89194(8)  | -15.89176(8)  | -15.89184(7)  |
| F                                               | -24.18514(7)  | -24.18515(7)  | -24.18527(7)  |
| Na                                              | -0.1821457(7) | -0.1821441(7) | -0.182145(2)  |
| Cl                                              | -14.97154(6)  | -14.97117(6)  | -14.97115(7)  |
| LiH                                             | -0.78787(3)   | -0.78800(2)   | -0.78799(1)   |
| BeH                                             | -1.58814(6)   | -1.58861(4)   | -1.58849(5)   |
| CH <sub>2</sub> ( <sup>3</sup> B <sub>1</sub> ) | -6.72719(9)   | -6.72762(7)   | -6.72777(8)   |
| LiF                                             | -24.60333(8)  | -24.60401(8)  | -24.60477(7)  |
| C <sub>2</sub> H <sub>2</sub>                   | -12.4878(1)   | -12.48906(9)  | -12.48920(7)  |
| CN                                              | -15.48083(8)  | -15.4833(1)   | -15.48371(8)  |
| HCN                                             | -16.20259(8)  | -16.20468(8)  | -16.20494(9)  |
| HCO                                             | -22.24632(9)  | -22.25065(8)  | -22.25173(9)  |
| NaCl                                            | -15.31021(6)  | -15.31104(8)  | -15.31135(7)  |

Table 12: The DMC total energies of the molecules from the G2 set and their atoms for a single determinant SJ trial wavefunction composed of VMC optimized orbitals. Energies are in Hartrees. Error bar, which is shown in parentheses, is for the last digit.

| System                                          | 2z            | 3z            | 5z            |
|-------------------------------------------------|---------------|---------------|---------------|
| H                                               | -0.5000005(1) | -0.5000006(1) | -0.5000005(1) |
| Li                                              | -0.1963295(4) | -0.1963292(4) | -0.1963296(3) |
| Be                                              | -1.00921(5)   | -1.00916(5)   | -1.00924(4)   |
| C                                               | -5.42244(6)   | -5.42258(5)   | -5.42245(5)   |
| N                                               | -9.79214(6)   | -9.79210(6)   | -9.79218(6)   |
| O                                               | -15.89241(9)  | -15.89249(7)  | -15.89272(7)  |
| F                                               | -24.18526(5)  | -24.18535(7)  | -24.18548(7)  |
| Na                                              | -0.1821438(7) | -0.1821446(4) | -0.1821438(4) |
| Cl                                              | -14.97209(6)  | -14.97204(6)  | -14.97212(5)  |
| LiH                                             | -0.78804(1)   | -0.78804(1)   | -0.788051(9)  |
| BeH                                             | -1.58833(4)   | -1.58887(3)   | -1.58883(3)   |
| CH <sub>2</sub> ( <sup>3</sup> B <sub>1</sub> ) | -6.72867(7)   | -6.72921(7)   | -6.72940(6)   |
| LiF                                             | -24.60451(8)  | -24.60473(8)  | -24.60479(8)  |
| C <sub>2</sub> H <sub>2</sub>                   | -12.4900(1)   | -12.49043(7)  | -12.49048(8)  |
| CN                                              | -15.49091(9)  | -15.49296(8)  | -15.49339(8)  |
| HCN                                             | -16.20593(8)  | -16.20711(7)  | -16.20741(7)  |
| HCO                                             | -22.25183(8)  | -22.25561(6)  | -22.25607(7)  |

Table 12 – continued

| System | 2z           | 3z           | 5z           |
|--------|--------------|--------------|--------------|
| NaCl   | -15.31167(5) | -15.31196(6) | -15.31202(7) |

Table 13: The DMC total energies of the molecules from the G2 set and their atoms for a CAS SJ trial wavefunction with an  $s$  and  $p$  active space. Energies are in Hartrees. Error bar, which is shown in parentheses, is for the last digit.

| System                                          | 3z            |
|-------------------------------------------------|---------------|
| H                                               | -0.5000006(1) |
| Li                                              | -0.1963292(4) |
| Be                                              | -1.010186(5)  |
| C                                               | -5.42775(5)   |
| N                                               | -9.79230(6)   |
| O                                               | -15.89305(8)  |
| F                                               | -24.18651(7)  |
| Na                                              | -0.1821446(4) |
| Cl                                              | -14.97252(6)  |
| LiH                                             | -0.788238(6)  |
| BeH                                             | -1.59014(2)   |
| CH <sub>2</sub> ( <sup>3</sup> B <sub>1</sub> ) | -6.73142(8)   |
| LiF                                             | -24.61011(7)  |
| C <sub>2</sub> H <sub>2</sub>                   | -12.50101(5)  |
| CN                                              | -15.50866(7)  |
| HCN                                             | -16.22003(6)  |
| HCO                                             | -22.26378(7)  |
| NaCl                                            | -15.31334(6)  |

## References

- [1] F R Petruzielo, Julien Toulouse, and C J Umrigar. Basis set construction for molecular electronic structure theory: Natural orbital and Gauss-Slater basis for smooth pseudopotentials. *J. Chem. Phys.*, 134(6):064104, 2011.
- [2] M. Burkatzki, C. Filippi, and M. Dolg. Energy-consistent pseudopotentials for quantum Monte Carlo calculations. *J. Chem. Phys.*, 126:234105, 2007.
- [3] <http://www.burkatzki.com/pseudos/index.2.html>.
- [4] Michael W. Schmidt, Jerry A. Boatz, Kim K. Baldridge, Steven T. Elbert, Mark S. Gordon, Jan H. Jensen, Shiro Koseki, Nikita Matsunaga, Kiet A. Nguyen, Shujun Su, Theresa L. Windus, Michel Dupuis, and John A. Montgomery. General atomic and molecular electronic structure system. *J. Comp. Chem.*, 14(11):1347–1363, 1993.
- [5] Larry A. Curtiss, Krishnan Raghavachari, Gary W. Trucks, and John A. Pople. Gaussian-2 theory for molecular energies of first- and second-row compounds. *J. Chem. Phys.*, 94(11):7221, 1991.
- [6] David Feller, Kirk A Peterson, and David A Dixon. A survey of factors contributing to accurate theoretical predictions of atomization energies and molecular structures. *J. Chem. Phys.*, 129(20):204105, 2008.
- [7] David Feller and Kirk A. Peterson. Re-examination of atomization energies for the Gaussian-2 set of molecules. *J. Chem. Phys.*, 110(17):8384, 1999.
- [8] Darragh P. O’Neill and Peter M. W. Gill. Benchmark correlation energies for small molecules. *Mol. Phys.*, 103(6-8):763–766, 2005.
- [9] Apostolos Kalamos, Thom H. Dunning Jr, and Aristides Mavridis. SiH<sub>2</sub>, a critical study. *Mol. Phys.*, (23-24):2597–2606, 2004.
- [10] R. D. Johnson, editor. *NIST Computational Chemistry Comparison and Benchmark Database, NIST Standard Reference Database Number 101*. NIST, Gaithersburg, MD, 2010.
- [11] Lubos Mitas, Eric L. Shirley, and David M. Ceperley. Nonlocal pseudopotentials and diffusion Monte Carlo. *J. Chem. Phys.*, 95(5):3467, 1991.
- [12] Michele Casula, Saverio Moroni, Sandro Sorella, and Claudia Filippi. Size-consistent variational approaches to nonlocal pseudopotentials: Standard and lattice regularized diffusion Monte Carlo methods revisited. *J. Chem. Phys.*, 132(15):154113, 2010.
